# Supplementary material for: Automated detection of pronunciation errors in non-native English speech employing deep learning
Source: arXiv:2209.06265 source file (2022-09-13)
Supplement: Supplementary file 1 [file 166_dk_wioleta.pdf]

POLITECHNIKA GDAŃSKA

The author of the doctoral dissertation: Daniel Korzekwa
Scientific discipline: Technical Informatics and Telecommunications

# DOCTORAL DISSERTATION

Title of doctoral dissertation: Automated detection of pronunciation errors in non-native English speech employing deep learning

Title of doctoral dissertation (in Polish): Automatyczna detekcja błędów wymowy z wykorzystaniem głębokiego uczenia maszynowego w celu wsparcia nauki języka

| | |
|---|---|
| Supervisor<br><br>*signature* | Second supervisor<br><br>*signature* |
| Prof. Bożena Kostek (Ph.D., D.Sc., Eng.) | <Title, degree, first name and surname> |
| Auxiliary supervisor<br><br>*signature* | Cosupervisor<br><br>*signature* |
| <Title, degree, first name and surname> | <Title, degree, first name and surname> |

Gdańsk, year 2022

POLITECHNIKA GDAŃSKA

# OPIS ROZPRAWY DOKTORSKIEJ

**Autor rozprawy doktorskiej**: Daniel Korzekwa

**Tytuł rozprawy doktorskiej w języku polskim**: Automatyczna detekcja błędów wymowy z wykorzystaniem głębokiego uczenia maszynowego w celu wsparcia nauki języka

**Tytuł rozprawy w języku angielskim**: Automated detection of pronunciation errors in non-native English speech employing deep learning

**Język rozprawy doktorskiej**: angielski

**Promotor rozprawy doktorskiej**: prof. dr hab. inż. Bożena Kostek

~~**Drugi promotor rozprawy doktorskiej***: <imię, nazwisko>~~

~~**Promotor pomocniczy rozprawy doktorskiej***: <imię, nazwisko>~~

~~**Kopromotor rozprawy doktorskiej***: <imię, nazwisko>~~

**Data obrony**:

**Słowa kluczowe rozprawy doktorskiej w języku polskim**: nauka wymowy wspomagana komputerowo, automatyczna detekcja błędów wymowy, synteza mowy, konwersja mowy, mowa dyzartryczna, głębokie uczenie maszynowe

**Słowa kluczowe rozprawy doktorskiej w języku angielskim**: computer-assisted pronunciation training, automated pronunciation error detection, speech synthesis, voice conversion, dysarthric speech, deep learning

**Streszczenie rozprawy w języku polskim**:

Pomimo znacznego postępu, jaki dokonał się w ostatnich latach, istniejące metody wspomaganego komputerowo treningu wymowy CAPT (ang. Computer-Assisted Pronunciation Training) wykrywają błędy wymowy ze stosunkowo niską dokładnością (precyzja rzędu 60% przy wskaźniku czułości 40%-80%). W niniejszej pracy doktorskiej zaproponowano nowe techniki głębokiego uczenia do wykrywania błędów wymowy w nierodzimej (L2) mowie angielskiej, przewyższając aktualny stan wiedzy w metryce wskaźnika pola AUC (Area under the Curve) o 41%, tj. z 0.528 do 0.749. Ze względu na małą dostępność baz adnotowanej mowy z błędami wymowy, potrzebnych do wiarygodnego treningu modeli głębokich, problem wykrywania błędów wymowy został przeformułowany na zadanie generowania syntetycznej mowy z błędami (L2) wymowy. W ten sposób w procesie syntezy mowy tworzone są dane treningowe do efektywnej detekcji błędów wymowy. Ponadto, aby wyeliminować potrzebę transkrypcji mowy nierodzimej na poziomie fonetycznym, zaproponowano nowatorską technikę wielozadaniową typu end-to-end do bezpośredniego wykrywania błędów wymowy. Opracowane modele zostały zastosowane w firmie Amazon do automatycznego wykrywania błędów wymowy w mowie syntetycznej w celu przyspieszenia badań nad nowymi technikami syntezy mowy. Pokazano, że zastosowane metody uczenia głębokiego aplikują się w zadaniach wykrywania i rekonstrukcji mowy dyzartrycznej.

**POLITECHNIKA GDAŃSKA**

**Streszczenie rozprawy w języku angielskim**:

Despite significant advances in recent years, the existing Computer-Assisted Pronunciation Training (CAPT) methods detect pronunciation errors with a relatively low accuracy (precision of 60% at 40%-80% recall). This Ph.D. work proposes novel deep learning methods for detecting pronunciation errors in non-native (L2) English speech, outperforming the state-of-the-art method in AUC metric (Area under the Curve) by 41%, i.e., from 0.528 to 0.749. One of the problems with existing CAPT methods is the low availability of annotated mispronounced speech needed for reliable training of pronunciation error detection models. Therefore, the detection of pronunciation errors is reformulated to the task of generating synthetic mispronounced speech. Intuitively, if we could mimic mispronounced speech and produce any amount of training data, detecting pronunciation errors would be more effective. Furthermore, to eliminate the need to align canonical and recognized phonemes, a novel end-to-end multi-task technique to directly detect pronunciation errors was proposed. The pronunciation error detection models have been used at Amazon to automatically detect pronunciation errors in synthetic speech to accelerate the research into new speech synthesis methods. It was demonstrated that the proposed deep learning methods are applicable in the tasks of detecting and reconstructing dysarthric speech.

** niepotrzebne skreślić*

*** dotyczy rozpraw doktorskich napisanych w innych językach, niż polski lub angielski*

GDAŃSK UNIVERSITY
OF TECHNOLOGY

# DESCRIPTION OF DOCTORAL DISSERTATION

**The Author of the doctoral dissertation**: Daniel Korzekwa

**Title of doctoral dissertation**: Automated detection of pronunciation errors in non-native English speech employing deep learning

**Title of doctoral dissertation in Polish**: Automatyczna detekcja błędów wymowy z wykorzystaniem głębokiego uczenia maszynowego w celu wsparcia nauki języka

**Language of doctoral dissertation**: English

**Supervisor**: Prof. Bożena Kostek (Ph.D., D.Sc., Eng.)

~~**Second supervisor***: <first name, surname >~~

~~**Auxiliary supervisior***: <first name, surname >~~

~~**Cosupervisior***: <first name, surname >~~

**Date of doctoral defense**:

**Keywords of doctoral dissertation in Polish**: nauka wymowy wspomagana komputerowo, automatyczna detekcja błędów wymowy, synteza mowy, konwersja mowy, mowa dyzartryczna, głębokie uczenie maszynowe

**Keywords of doctoral dissertation in English**: computer-assisted pronunciation training, automated pronunciation error detection, speech synthesis, voice conversion, dysarthric speech, deep learning

**Summary of doctoral dissertation in Polish**:

Pomimo znacznego postępu, jaki dokonał się w ostatnich latach, istniejące metody wspomaganego komputerowo treningu wymowy CAPT (ang. Computer-Assisted Pronunciation Training) wykrywają błędy wymowy ze stosunkowo niską dokładnością (precyzja rzędu 60% przy wskaźniku czułości 40%-80%). W niniejszej pracy doktorskiej zaproponowano nowe techniki głębokiego uczenia do wykrywania błędów wymowy w nierodzimej (L2) mowie angielskiej, przewyższając aktualny stan wiedzy w metryce wskaźnika pola AUC (Area under the Curve) o 41%, tj. z 0.528 do 0.749. Ze względu na małą dostępność baz adnotowanej mowy z błędami wymowy, potrzebnych do wiarygodnego treningu modeli głębokich, problem wykrywania błędów wymowy został przeformułowany na zadanie generowania syntetycznej mowy z błędami (L2) wymowy. W ten sposób w procesie syntezy mowy tworzone są dane treningowe do efektywnej detekcji błędów wymowy. Ponadto, aby wyeliminować potrzebę transkrypcji mowy nierodzimej na poziomie fonetycznym, zaproponowano nowatorską technikę wielozadaniową typu end-to-end do bezpośredniego wykrywania błędów wymowy. Opracowane modele zostały zastosowane w firmie Amazon do automatycznego wykrywania błędów wymowy w mowie syntetycznej w celu przyspieszenia badań nad nowymi technikami syntezy mowy. Pokazano, że zastosowane metody uczenia głębokiego aplikują się w zadaniach wykrywania i rekonstrukcji mowy dyzartrycznej.

GDAŃSK UNIVERSITY OF TECHNOLOGY


**Summary of doctoral dissertation in English**:

Despite significant advances in recent years, the existing Computer-Assisted Pronunciation Training (CAPT) methods detect pronunciation errors with a relatively low accuracy (precision of 60% at 40%-80% recall). This Ph.D. work proposes novel deep learning methods for detecting pronunciation errors in non-native (L2) English speech, outperforming the state-of-the-art method in AUC metric (Area under the Curve) by 41%, i.e., from 0.528 to 0.749. One of the problems with existing CAPT methods is the low availability of annotated mispronounced speech needed for reliable training of pronunciation error detection models. Therefore, the detection of pronunciation errors is reformulated to the task of generating synthetic mispronounced speech. Intuitively, if we could mimic mispronounced speech and produce any amount of training data, detecting pronunciation errors would be more effective. Furthermore, to eliminate the need to align canonical and recognized phonemes, a novel end-to-end multi-task technique to directly detect pronunciation errors was proposed. The pronunciation error detection models have been used at Amazon to automatically detect pronunciation errors in synthetic speech to accelerate the research into new speech synthesis methods. It was demonstrated that the proposed deep learning methods are applicable in the tasks of detecting and reconstructing dysarthric speech.


**delete where appropriate*

***applies to doctoral dissertations written in other languages, than Polish or English*

GDAŃSK UNIVERSITY OF TECHNOLOGY

**THE "IMPLEMENTATION DOCTORATE" PROGRAM OF THE MINISTER OF EDUCATION AND SCIENCE AT GDANSK UNIVERSITY OF TECHNOLOGY**

This Ph.D. was conducted within the framework of the "Implementation Doctorate" Program of the Ministry of Education and Science at Gdansk University of Technology, under the supervision of prof. Bożena Kostek (Gdańsk University of Technology) and Roberto Barra-Chicote, Ph.D. (TTS Research, Amazon).
